# Supplementary material for: Effect of quantum Hall edge strips on valley splitting in silicon quantum wells
Source: arXiv:2006.02305 source file (2020-09-29)
Supplement: Supplementary file 1 [file PaqueletWuetz_suppl.pdf]

# Supplemental Material for "Effect of quantum Hall edge strips on valley splitting in silicon quantum wells"

Brian Paquelet Wuetz,[1] Merritt P. Losert,[2] Alberto Tosato,[1] Mario Lodari,[1] Peter L. Bavdaz,[1] Lucas Stehouwer,[1] Payam Amin,[3] James S. Clarke,[3] Susan N. Coppersmith,[4] Amir Sammak,[5] Menno Veldhorst,[1] Mark Friesen,[2] and Giordano Scappucci[1,*]

[1] *QuTech and Kavli Institute of Nanoscience, Delft University of Technology, PO Box 5046, 2600 GA Delft, The Netherlands*
[2] *University of Wisconsin-Madison, Madison, WI 53706 USA*
[3] *Components Research, Intel Corporation, 2501 NW 229th Ave, Hillsboro, OR 97124, USA*
[4] *University of New South Wales, Sydney, Australia*
[5] *QuTech and Netherlands Organisation for Applied Scientific Research (TNO), Stieltjesweg 1, 2628 CK Delft, The Netherlands*

## I. ANALYSIS OF HIGH-ANGLE ANNULAR DARK FIELD SCANNING TRANSMISSION ELECTRON MICROSCOPY INTENSITY PROFILE

In Fig. S1 we show the intensity profile from high angle annular dark field scanning transmission electron microscopy (HAADF-STEM) along $z$, the heterostructure growth direction, and a theoretical fit to the function $erf(\frac{z-z_0}{\sqrt{2}\lambda})$. Erf is the error function, $z_0$ is the center of the quantum well top-interface, where the HAADF-STEM intensity signal is midway in between the value measured at the quantum well and at the SiGe barrier, and $\lambda$ is the characteristic distance. The HAADF-STEM intensity signal is shown after a linear background subtraction and normalization to the value measured in the quantum well. We extract $\lambda = 1.04 \pm 0.03$ nm from the fit.

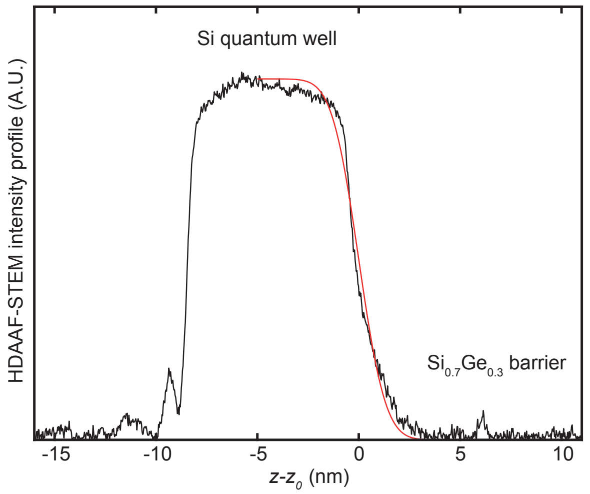


Figure S1. HAADF-STEM intensity profile (black line) along the $z$, the heterostructure growth direction. The red line is a theoretical fit of the data in the region corresponding to the top interface between the Si quantum well and the SiGe barrier (see text for details). For clarity, the horizontal axis is offset by $z_0$, the coordinate of the center of the quantum well top interface

## II. G-FACTOR ANALYSIS

We determine the $g$-factor from the thermally activated dependence of the Shubnikov de Haas (SdH) oscillation minimum for spin split levels[1]. Figure S2 shows the mobility gaps for Zeeman spin split levels ($\Delta_Z$, blue circles) and valley split levels ($\Delta_v$, red cirles) as a function of magnetic field. Similarly to the procedure described in the main text, these data points are obtained by fitting the temperature dependent magnetoresistance oscillation minima in the density range of (0.9–4) $\times$ $10^{11}$ $cm^{-2}$ to an Arrhenius law $\rho_{xx} \propto \exp(-\Delta_Z/2k_BT)$ and $\rho_{xx} \propto \exp(-\Delta_v/2k_BT)$ for spin and valley states, respectively. Both $\Delta_Z$ and $\Delta_v$ increase linearly with magnetic field. Taking into account the reduction of the Zeeman energy gap $g\mu_BB$ due to valley splitting $E_v = c_BB$ and Landau level broadening $\Gamma$ (see inset in Fig. S2), the linear increase of $\Delta_Z$ and $\Delta_v$ with magnetic field is described by the following two equations:

$$\Delta_Z = g\mu_BB - c_BB - \Gamma \tag{1}$$

$$\Delta_v = c_BB - \Gamma \tag{2}$$

We fit the experimental points $\Delta_Z$ and $\Delta_v$ in Fig. S2 to Eq 1. and 2. using $g$, $c_B$ and $\Gamma$ as fitting parameters. We extract: $g = 1.8 \pm 0.05$, $c_B = 27.5 \pm 0.9$ $\mu$eV/T and $\Gamma = 35.3 \pm 3.3$ $\mu$eV. The obtained values of $c_B$ and $\Gamma$ are compatible with the analysis in the main text. The solid lines in Fig S2 correspond to the Zeeman energy $g^*\mu_BB$ and valley splitting energy $E_v = c_BB$, taking into account $\Gamma$. The $g$-factor $\approx$ 1.8 is close and not greater than the single particle value $g = 2$, suggesting that the measured quantum Hall gaps in the main text are not enhanced by electron-electron interaction and thus represent single-particle energy gaps.

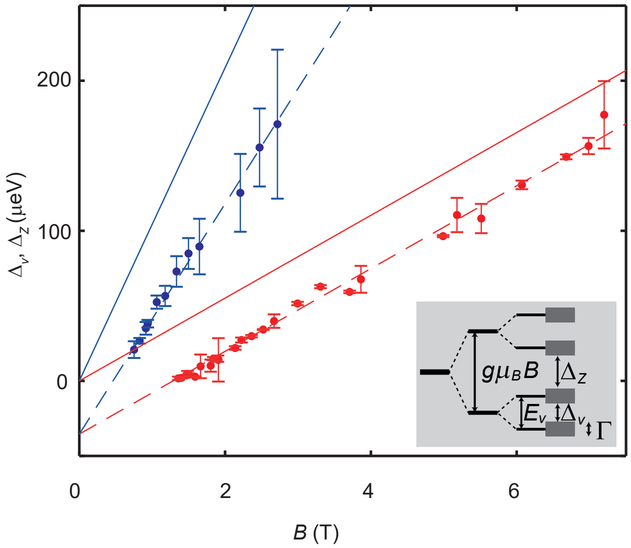


Figure S2. Mobility gaps obtained from thermal activation of Shubnkiov de Haas oscillation minima for $2n$ - 1 fillings factors ($\Delta_v$, red circles) and $4n$ - 2 filling factors ($\Delta_Z$, blue circles), corresponding to valley and Zeeman split levels, respectively. The blue and red dashed lines are theoretical fits to the experimental data using equations (1) and (2), respectively. The blue and red solid lines correspond to the estimated Zeeman and valley energy gaps, respectively. The inset shows splitting of a Landau level due to Zeeman spin splitting and valley splitting. Shaded areas represent the single-particle level broadening Γ due to disorder.

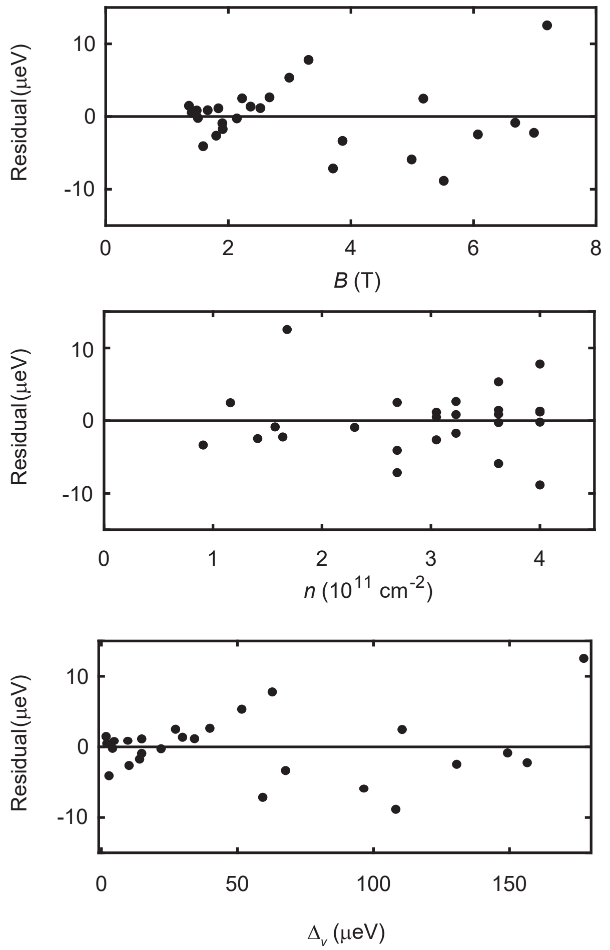


Figure S3. Residual plot of the activation energy $\Delta_v$ reported in Fig. 2 to the plane defined by the equation $\Delta_v = c_B B + c_n n - \Gamma$ with $c_B = 28.1$ $\mu$eV/T, $c_n = 0.1$ $\mu$eV/$10^{11}$cm$^{-2}$, and $\Gamma = 37.5$ $\mu$eV. Residuals are plotted as a function of (a) magnetic field $B$, (b) Hall density, (c) activation energy $\Delta_v$.

## III. RESIDUALS FOR THE PLANAR FIT OF $\Delta_V$ AS A FUNCTION OF MAGNETIC FIELD AND HALL DENSITY

In Fig. S3 we show the residuals to highlight the agreement between experimental data points and theoretical fit in Fig. 2 of the main text. For clarity, the residuals are plotted against magnetic field $B$ (Fig. S3 (a)), Hall density (Fig. S3 (b)), and activation energy $\Delta_v$ (Fig. S3 (c)). Overall we observe small residuals with random distributions around zero, indicating a good fit.

## IV. THEORETICAL METHODS

Figure 3 of the main text presents theoretical estimates for the valley splitting as a function of the magnetic field, $B$, and the two-dimensional electron density, $n$. This Supplementary Section presents details of the calculations.

The final goal of the simulation procedure is to determine the vertical electric field in the quantum Hall edge states. As a first step, we calculate the energy of a two-dimension electron gas (2DEG), which has two predominant contributions. The first is electrostatic, arising from voltages applied to top-gates, and electron-electron interactions in the 2DEG that yield screening. The second is from vertical confinement of the 2DEG (perpendicular to the 2DEG), caused by the quantum well and the vertical electric field. In the quantum Hall regime, the density of states in the 2DEG splits into highly degenerate quantized levels; however, these energy splittings are significantly smaller than the electrostatic and vertical confinement energies[2]. This separation of energy scales allows the vertical and lateral confinement problems to be solved independently, via the Born-Oppenheimer approximation, and it also allows us to apply Thomas-Fermi quasiclassical methods to describe the electrostatic screening[2]. Below, we combine the Born-Oppenheimer and Thomas-Fermi methods in a single self-consistent scheme.

For a 2DEG, the Born-Oppenheimer approximation allows us to treat the vertical ($z$) and lateral ($x$-$y$) confine-

ment problems independently, beginning with the former. The vertical confinement and the electrostatics can be solved simultaneously and self-consistently using the Hartree approximation[3]. The full three-dimensional (3D) electron density takes the form $n_{3D} \approx |\psi(z)|^2 n(x,y)$, where $\psi$ is the vertical (one-dimensional) wavefunction, and $n$ is the usual 2D electron density. Note that $\psi(z)$ depends implicitly on $x$ and $y$ through $n$, which is taken to be a constant in this calculation. Since the electric fields used to accumulate electrons in a 2DEG are quite large, we use the method described in Ref.[4] to include important corrections arising from the wavefunction penetration into the quantum well barrier. At low temperatures, we find that electrons are confined to the lowest quantum well subband with a confinement energy given by

$$E_{\rm sb} = \frac{5}{16}\left(\frac{33}{2}\right)^{2/3}\left[\frac{\hbar^2}{2m_l}\left(\frac{e^2 n}{\epsilon}\right)^2\right]^{1/3} - \frac{5}{3}\sqrt{\frac{2}{33}}\frac{e^2 n}{\epsilon}\sqrt{\frac{\hbar^2}{m_l \Delta E_c}}, \quad (3)$$

where $m_l \simeq 0.92 m_0$ is the longitudinal effective mass in silicon, $\epsilon \simeq 11.4\epsilon_0$ is the dielectric constant in low-temperature silicon, and $\Delta E_c$ is the conduction band offset of the $\mathrm{Si}_{1-x}\mathrm{Ge}_x/\mathrm{Si}/\mathrm{Si}_{1-x}\mathrm{Ge}_x$ quantum well, which we take to be $\Delta E_c = 0.15$ eV for the $x = 0.3$ heterostructures used in this experiment. The first term in Eq. (3) is the leading-order contribution from confinement in an approximately triangular quantum well. The second term is the correction for the penetration of the electron wavefunction into the SiGe barrier.

Next we solve the full, 3D electrostatics, taking into account the lateral variations of $n(x,y)$. In this case, we treat the 2DEG as strictly two-dimensional, in a plane located 2 nm below the top of the quantum well. In the Thomas-Fermi method, the electron density $n(x,y)$ and the electrostatic potential $\phi(x,y,z)$ are determined self-consistently. Typically[5], $n$ is determined by integrating the density of states, from the lowest available electron energy in the conduction band ($-e\phi$) up to the Fermi level, $E_F$, which corresponds to the global chemical potential. Here, we use the same method, but we replace the lower limit of the integration with the full quasiclassical energy, $-e\varphi + E_{\rm sb}$. The resulting Thomas-Fermi approximation for the 2DEG density is given by

$$n = \frac{g_{\rm Si} m_t}{2\pi\hbar^2}(E_F + e\varphi - E_{\rm sb})\Theta[E_F + e\varphi - E_{\rm sb}], \quad (4)$$

where $g_{\rm Si} = 4$ is the band degeneracy factor for strained silicon, including two spin and two valley degrees of freedom, $m_t \simeq 0.19 m_0$ is the transverse effective mass, and $\Theta[\cdot]$ is the Heaviside step function.

Several of the terms in Eq. (4) depend on $n$. However, the term originating from the first term in Eq. (3), which is proportional to $n^{2/3}$, is considerably larger than the others. It is therefore convenient to adopt an approximation of the form

$$n \simeq \frac{3n_t^{1/3} n^{2/3}}{2} - \frac{n_t}{2} \quad (5)$$

for the smaller, linear-in-$n$ terms in Eq. (4), which is valid for $n \simeq n_t$, where $n_t$ is a typical value of the electron density. In practice, we find that Eq. (5) provides accurate results over the entire experimental range of interest when choosing $n_t = 2 \times 10^{11}$ cm$^{-2}$. Rearranging terms, the improved Thomas-Fermi approximation can be rewritten as

$$\frac{n}{n_t} = \left[\frac{E_F + e\varphi}{\frac{3\pi\hbar^2 n_t}{4m_t} - \frac{5e^2 n_t}{2\epsilon}\sqrt{\frac{2\hbar^2}{33 m_l \Delta E_c}} + \frac{5}{32}\left(\frac{\hbar^2}{m_l}\right)^{1/3}\left(\frac{33 e^2 n_t}{\epsilon}\right)^{2/3}}\right]^{3/2} \Theta\left[E_F + e\varphi\right], \quad (6)$$

where we have absorbed a global constant into the definition of $E_F$. For the parameters assumed here, this simplifies to

$$n = 1.6 \times 10^{46}(E_F + e\varphi)^{3/2}\Theta[E_F + e\varphi], \quad (7)$$

where we have assumed SI units. It is interesting to note that the scaling dependence $n \sim (E_F + e\varphi)^{3/2}$ observed in Eq. (7) is consistent with the 3D Thomas-Fermi approximation. This is a natural outcome of accounting for the confinement energy in Eq. (3), which arises from the third spatial dimension, perpendicular to the 2DEG. Since this confinement energy is relatively large, and depends strongly on $n$, it suggests that the more conventional 2D Thomas-Fermi approximation is likely to yield inaccurate results.

The Fermi level $E_F$ appearing in Eq. (7) is constant across the whole sample, and its value is chosen to yield the desired electron density in the bulk region. For our activation energy experiments, the bulk density is given by $n_{\rm bulk} = \nu_{\rm bulk} n_B$, where $n_B = eB/h$ is the density of a single filled level[2], and $\nu_{\rm bulk}$ is an integer. The values of $n$ reported in the figures in the main text correspond to $n = n_{\rm bulk}$. However, the theoretical valley splittings reported in the main text are obtained from the same simulations by evaluating the vertical electric field $E_z$ in the outer edge channel, at the position where $n = n_B$.

Finally, for completeness, we present the full energy of a 2DEG in the quantum Hall regime, including lateral quantization effects, although it is not used in our simulations:

$$\varepsilon(n, B, n_{\mathrm{LL}}, m_s, m_v) = -e\varphi(x, y) + E_{\mathrm{sb}}(x, y) + (n_{\mathrm{LL}} + \frac{1}{2})\frac{e\hbar B}{m_t} + m_s g^* \mu_B B + m_v E_v. \quad (8)$$

Here, $n_{\mathrm{LL}} = 0, 1, 2, \ldots$ is the Landau level index, $m_s = \pm 1/2$ is the spin quantum number, $g^*$ is the Landé $g$-factor, $m_v = \pm 1/2$ is the valley quantum number, and $E_v$ is the valley splitting.

* g.scappucci@tudelft.nl

[1] S. F. Neyens, R. H. Foote, B. Thorgrimsson, T. J. Knapp, T. McJunkin, L. M. K. Vandersypen, P. Amin, N. K. Thomas, J. S. Clarke, D. E. Savage, M. G. Lagally, M. Friesen, S. N. Coppersmith, and M. A. Eriksson, Applied Physics Letters **112**, 243107 (2018).

[2] D. B. Chklovskii, B. I. Shklovskii, and L. I. Glazman, Physical Review B **46**, 4026 (1992).

[3] J. H. Davies, *The Physics of Low-dimensional Semiconductors: An Introduction* (Cambridge University Press, 1998).

[4] M. Friesen, S. Chutia, C. Tahan, and S. N. Coppersmith, Physical Review B **75**, 115318 (2007).

[5] A. Frees, J. K. Gamble, D. R. Ward, R. Blume-Kohout, M. Eriksson, M. Friesen, and S. Coppersmith, Physical Review Applied **11**, 024063 (2019).
